# Supplementary material for: Jam Sessions: Analysis and Experimental Evaluation of Advanced Jamming Attacks in MIMO Networks
Source: arXiv:1904.07613 source file (2019-04-16)
Supplement: Supplementary file 1 [file appendix.tex]

% \appendix

% \vspace{-2mm}
% \section{Proof of Lemma \ref{lem1}}
% % Since $\mb{E} \{\tilde{H}\} = \mf{0}_{N \times M}$ is obvious,  we will focus on $\mb{E} \{\tilde{H} A \tilde{H}\}$. With the optimal training sequence $X X^H = K E_s I_M$, we have
% % \begin{equation}
% % 	\begin{split}
% % 		\mb{E} \{\tilde{H} A \tilde{H}^H\} = & \mb{E} \{(GZ + W) X^{\dagger} A 
% % (X^{\dagger})^H (GZ + W)^H \} \\
% % 		= & \frac{1}{K^2 E_s^2} \mb{E}\{(GZ + W) X^H A X (GZ + W)^H\} \\
% % 		= & \frac{1}{K^2 E_s^2} \left( \mb{E}\{ GZ X^H A X Z^HG^H \} \right. \\
% % 		& \left. + \mb{E}\{ W X^H A X W^H \} \right) \\
% % 		= & \frac{1}{K^2 E_s^2} \left( D B D^H + W B W^H \right),
% % 	\end{split}
% % \end{equation}
% % where we denote $D = GZ$, and $B = X^H A X$.

% % For the interference $D$, we have
% % \begin{equation}
% % 	\begin{split}
% % 		D & = G Z \\
% % 		& = \left[
% % 			\begin{array}{ccc}
% % 				g_{11} & \cdots & g_{1L} \\
% % 				\vdots & \ddots & \vdots \\
% % 				g_{N1} & \cdots & g_{NL}
% % 			\end{array}
% % 		\right] \cdot \left[
% % 			\begin{array}{ccc}
% % 				z_{11} & \ldots & z_{1K} \\
% % 				\vdots & \ddots & \vdots \\
% % 				z_{L1} & \ldots & z_{LK}
% % 			\end{array}
% % 		\right] \\
% % 		& = \left[
% % 			\begin{array}{ccc}
% % 				\sum_l g_{1l} z_{l1} & \ldots & \sum_l g_{1l} z_{lK} \\
% % 				\vdots & \ddots & \vdots \\
% % 				\sum_l g_{Nl} z_{l1} & \ldots & \sum_l g_{Nl} z_{lK}
% % 			\end{array}
% % 		\right] \\
% % 		& \triangleq \left( \mf{d}_1, \ldots, \mf{d}_K \right).
% % 	\end{split}
% % 	\vspace{-2mm}
% % \end{equation}
% % Column $k$ of $Z$ represents the jamming signal at time instant $k$. Therefore, they are mutually independent. Consequently, the columns of $D$ are also uncorrelated, and
% % \begin{equation}
% % 	\mb{E} \{\mf{d}_k \mf{d}_{k'}^H\} = \left\{
% % 		\begin{array}{ll}
% % 			E_j GG^H, & k = k', \\
% % 			\mf{0}_{N \times N}, & k \ne k'.
% % 		\end{array}
% % 	\right.
% % \end{equation}

% % Therefore,

% % \vspace{-2mm}
% % \begin{equation}
% % 	\begin{split}
% % 		\mb{E} \{ D B D^H\} 
% % 		= & \mb{E} \left\{ (\mf{d}_1, \ldots, \mf{d}_K) \cdot \left[
% % 			\begin{array}{ccc}
% % 				b_{11} & \ldots & b_{1K} \\
% % 				\vdots & \ddots & \vdots \\
% % 				b_{K1} & \ldots & b_{KK}
% % 			\end{array}
% % 		\right] \right. \left. \cdot \left(
% % 			\begin{array}{c}
% % 				\mf{d}_1^H \\
% % 				\vdots \\
% % 				\mf{d}_K^H
% % 			\end{array}
% % 		\right) \right\} \\
% % 		= & \mb{E} \left\{\sum_k b_{kk} \mf{d}_k \mf{d}_k^H\right\} =  E_j \mr{tr}(B) GG^H.
% % 	\end{split}
% % 	\vspace{-2mm}
% % \end{equation}


% % Since $B = X^H A X$, we have $\mr{tr}(B) = \mr{tr}(X^H A X) = \mr{tr}(X X^H A) = K E_s \mr{tr}(A)$
% % and $\mb{E} \{D B D^H\} = E_j K E_s \mr{tr}(A) GG^H$.


% % For the term $WBW^H$, since all the entries of $W$ are i.i.d, we have
% % \begin{equation}
% % 	\mb{E} \{W B W^H\} = N_0 \mr{tr}(B) = N_0 K E_s \mr{tr}(A) I_N.
% % \end{equation}

% % Therefore,
% % \begin{equation}
% % 	\mb{E} \{\tilde{H} A \tilde{H}^H\} = \frac{1}{K E_s} \mr{tr}(A) \left( E_j GG^H + N_0 I_N \right).
% % \end{equation}

% \section{Proof of Lemma \ref{lem2}}
%     The autocorrelation can be derived as follows:
% \begin{equation}
% 	\begin{split}
% 		\mb{E} \{\hat{\mf{w}}\hat{\mf{w}}^H\} = & \mb{E} \{(H^{\dagger} \mf{w} - H^{\dagger} \tilde{H} \mf{x} - H^{\dagger} \tilde{H} H^{\dagger} \mf{w}) \\
% 		& \cdot (H^{\dagger} \mf{w} - H^{\dagger} \tilde{H} \mf{x} - H^{\dagger} \tilde{H} H^{\dagger} \mf{w})^H\} \\
% 		=~& \mb{E} \{ H^{\dagger} \mf{w} \mf{w}^H (H^{\dagger})^H + H^{\dagger} \tilde{H} \mf{x} \mf{x}^H \tilde{H}^H (H^{\dagger})^H \\
% 		& + H^{\dagger} \tilde{H} H^{\dagger} \mf{w} \mf{w}^H (H^{\dagger})^H \tilde{H}^H (H^{\dagger})^H \} \\
% 		=~& N_0 (H^HH)^{-1} + \frac{M}{K} H^{\dagger} \left( E_j GG^H + N_0 I_N \right) (H^{\dagger})^H \\
% 		& + \frac{N_0}{KE_s} \mr{tr}( (H^HH)^{-1} ) H^{\dagger} ( E_j GG^H + N_0 I_N ) (H^{\dagger})^H
% 	\end{split}
% \end{equation}

% According to \cite{Wang2007TWC}, $\mr{tr}((H^HH)^{-1})$ is a small value typically no larger than $M$. Since we are focusing on high SNR (by SNR we mean signal to noise ratio, the SIR or SJR is not necessarily high) scenario, this implies that $\sfrac{N_0}{E_s} \mr{tr}((H^HH)^{-1}) << M$. In other words, the last term is much smaller than the second term and can be neglected. Therefore, we have
% \begin{equation}
% 	\mb{E} \{\hat{\mf{w}}\hat{\mf{w}}^H\} \approx \left(1 + \frac{1}{K}\right) N_0 (H^HH)^{-1} + \frac{E_j}{K} H^{\dagger} GG^H (H^{\dagger})^H.
% \end{equation}
